# Supplementary material for: Quantum State Discrimination Using the Minimum Average Number of Copies
Source: arXiv:1605.07807 ancillary file (2017-02-20)
Supplement: Supplementary file 1 [file GOFdiscr_SM_v15.pdf]

# Quantum state discrimination using the minimum average number of copies: Supplemental Material

Sergei Slussarenko,[1] Morgan M. Weston,[1] Jun-Gang Li,[1,2] Nicholas Campbell,[1] Howard M. Wiseman,[1,*] and Geoff J. Pryde[1,†]

[1]*Centre for Quantum Dynamics and Centre for Quantum Computation and Communication Technology, Griffith University, Brisbane, Queensland 4111, Australia*

[2]*School of Physics, Beijing Institute of Technology, Beijing 100081, China*

(Dated: December 22, 2016)

We provide details on: (I) derivation of cost functions $C^{\rm FBM}(\varepsilon)$ and $C^{\rm LOL}(\varepsilon)$ and the random walk-based approach for the cost function $C^{\rm UBM}(\varepsilon)$; (II) optimal measurement angles and the asymptotic behavior of discrimination strategies within the guaranteed bounded error discrimination task; and (III) experimental setup characterization and calibration.

## I. DERIVATION OF COST FUNCTIONS

We consider the case when $n$ copies of identical quantum systems that exist in one of two possible nonorthogonal pure states $|\psi_j\rangle = \cos\theta|x\rangle - (-1)^j \sin\theta|y\rangle$, with $j = 1, 2$ and $\theta \in (0, \pi/4)$, for some orthonormal basis $\{|x\rangle, |y\rangle\}$. The states are prepared with probabilities $q_1$ and $q_2$ and without loss of generality, we assume $q_1 \geq q_2$. The general measurement we can perform on the system is a positive operator-valued measure, i.e. a pair of positive operators $\hat{E}_1$ and $\hat{E}_2$ such that $\hat{E}_1 + \hat{E}_2 = \hat{I}$, where $\hat{I}$ is the identity operator. For the $n$-th local measurement the conditional probability of obtaining a result $D_n (D = 1, 2)$ given the state $|\psi_j\rangle$ $(j = 1, 2)$ is $p(D_n|\psi_j) = {\rm Tr}[|\psi_j\rangle\langle\psi_j|\hat{E}_{D_n}]$. In case of projective measurements, $\hat{E}_D = |\varphi_D\rangle\langle\varphi_D|$, this probability reduces to

$$p(D_n|\psi_j) = \cos^2\left(\varphi - \frac{\pi}{2}(D_n - 1) + (-1)^j\theta\right). \tag{S1}$$

Note that $\varphi_n$ can change with $n$ and in fact for adaptive measurements can be a function of the prior string of measurement outcomes $\chi_{n-1} = D_1 D_2 \cdots D_{n-1}$. Then the posterior probability $p_n$ of the quantum system being in the state $|\psi_1\rangle$ after a particular string $\chi_n$ of local measurement outcomes was observed can be calculated using Bayes theorem

$$p_n(\psi_1|\chi_n) = \frac{p_{n-1}(\psi_1|\chi_{n-1})p(D_n|\psi_1)}{p_{n-1}(\psi_1|\chi_{n-1})p(D_n|\psi_1) + [1 - p_{n-1}(\psi_1|\chi_{n-1})]p(D_n|\psi_2)}. \tag{S2}$$

The update of the posterior probability after a $n$-th local measurement depends on prior string $\chi_{n-1}$ and in order to calculate $p_n(\psi_1|\chi_n)$ explicitly, the recursive Eq. (S2) has to be followed, starting with $p_0(\psi_1|\chi_0) = q_1$. We note that Bayesian analysis is not limited to pure states and can be applied when $\rho_j$ are mixed.

Expanding Eq. (S1) to a string of measurement outcomes $\chi_n$ will give us: $p_n(\chi_n|\psi_j) = p(D_1|\psi_j)\cdots p(D_n|\psi_j)$ the conditional probabilities of obtaining outcome string $\chi_n$ if the state is $|\psi_j\rangle$. Thus $P(\chi_n) = q_1 p(\chi_n|\psi_1) + q_2 p(\chi_n|\psi_2)$ is the probability of observing a $\chi_n$ string, if $n$ measurements were performed. In terms of these, Eq. (S2) evaluates to

$$p_n(\psi_1|\chi_n) = \frac{q_1 p(\chi_n|\psi_1)}{P(\chi_n)}, \tag{S3}$$

as the posterior probability of the system to be in state $|\psi_1\rangle$, given the measurement string is $\chi_n$. The probability of erroneous discrimination with an outcome string $\chi_n$ is then given by [1]

$$P({\rm err}|\chi_n) = \min\{p_n(\psi_1|\chi_n), 1 - p_n(\psi_1|\chi_n)\}. \tag{S4}$$

We can now define both the average discrimination error given $n$ number of copies (to be minimized in the minimum-error discrimination task)

$$E_n = \sum_{\chi_n} P(\chi_n)P({\rm err}|\chi_n), \tag{S5}$$

* h.wiseman@griffith.edu.au
† g.pryde@griffith.edu.au

and average number of resources, required to reach a pre-set error bound $\varepsilon$ (to be minimized in the guaranteed bounded error discrimination task)

$$C(\varepsilon) = \sum_{n=1}^{\infty} \left[ n \sum_{\chi_n} P(\chi_n)\mathcal{H}(\chi_n) \right], \tag{S6}$$

where $\mathcal{H}(\chi_n)$ is defined as

$$\mathcal{H}(\chi_n) = \begin{cases} 1 & \text{if } P(\text{err}|\chi_n) \le \varepsilon \text{ and } P(\text{err}|\chi_{n'}) > \varepsilon, n' < n \\ 0 & \text{otherwise.} \end{cases} \tag{S7}$$

If we restrict ourselves to $X_n \in \mathbb{S}_n (n = 1..\infty)$, i.e only those detection strings that lead to a conclusive discrimination result, Eq. (S6) reduces to

$$C(\varepsilon) = \sum_{n=1}^{\infty} n \sum_{X_n \in \mathbb{S}_n} P(X_n). \tag{S8}$$

*1. Fully biased measurement.* In the FBM strategy, we set $\varphi = \theta$. In this case the conditional probabilities (S1) and the posterior probability (S3) of the state being in $|\psi_1\rangle$, given the outcome string $\chi_n$ depend only on the number $m$ of $D = 1$ outcomes (corresponding to $|\varphi_1\rangle$) in the string $\chi_n$. The number of $D = 2$ outcomes (corresponding to $|\varphi_2\rangle$) is of course $n - m$. Denoting $\chi_n^m$ as a measurement string with $m$ outcomes $D = 1$, the formulae are

$$p(1|\psi_1) = 1,\ p(1|\psi_2) = \cos^2 2\theta,\ p(2|\psi_1) = 0,\ p(2|\psi_2) = \sin^2 2\theta, \tag{S9}$$

and

$$p_n(\psi_1|\chi_n^m) = \frac{q_1[p(1|\psi_1)]^m[p(2|\psi_1)]^{n-m}}{q_1[p(1|\psi_1)]^m[p(2|\psi_1)]^{n-m} + q_2[p(1|\psi_2)]^m[p(2|\psi_2)]^{n-m}} = \begin{cases} g(n) & \text{if } m = n, \\ 0 & \text{if } m < n \end{cases} \tag{S10}$$

respectively, where $g(n) = q_1(q_1 + q_2\cos^{2n} 2\theta)^{-1}$. The probability of error with an outcome string $\chi_n^m$ is then given by

$$P(\text{err}|\chi_n^m) = \begin{cases} g(n) & \text{if } m = n, \\ 0 & \text{if } m < n. \end{cases} \tag{S11}$$

Since $g(n)$ is a monotonically decreasing function of $n$, for a pre-set $\varepsilon$ we easily find that the number of copies required to satisfy the condition

$$P(\text{err}|\chi_n^m) \le \varepsilon. \tag{S12}$$

for all values of $m$ is

$$n_T = \left\lceil \frac{\ln(q_1\varepsilon) - \ln[q_2(1-\varepsilon)]}{2\ln(\cos 2\theta)} \right\rceil. \tag{S13}$$

In the guaranteed bounded error discrimination task, the measurement protocol continues until $n_T$ outcomes $D = 1$ are observed, corresponding to a discrimination $|\psi_1\rangle$, unless at least one $D = 2$ outcome appears, terminating the measurement immediately with the result $|\psi_2\rangle$. Thus, the set of observable measurement strings $X_n$ is formed by the string $1_1...1_{n_T}$ and by the set of strings of the form $1_1...1_{n-1}2_n$ with $n \le n_T$. The probabilities of observing these measurement strings are

$$\mathcal{P}_1(n) = P(1_1...1_n) = q_1 + q_2\cos^{2n} 2\theta \tag{S14}$$

and

$$\mathcal{P}_2(n) = P(1_1...1_{n-1}2_n) = q_2\sin^2 2\theta\cos^{2n} 2\theta, \tag{S15}$$

respectively.

Using Eq. (S8) here we can now derive the cost function as

$$\begin{aligned} C^{\text{FBM}}(\varepsilon) &= \sum_{n=1}^{n_T} n\mathcal{P}_2(n) + n_T\mathcal{P}_1(n_T) \\ &= q_1 n_T + q_2 \frac{1-(\cos 2\theta)^{2n_T}}{\sin^2 2\theta}. \end{aligned} \tag{S16}$$

*2. Locally optimal local measurement.* In the LOL strategy the measurement angle $\varphi$ for each subsequent measurement depends on the outcome of the previous one. An $n$-th measurement is a Helstrom measurement with prior probability set as the $(n-1)$-th posterior probability. The probability of error given the outcomes $\chi_n$ can be written as [2]

$$P(\text{err}|\chi_n) = \frac{1}{2}\left(1 - \sqrt{1 - 4q_1 q_2 \cos^{2n} 2\theta}\right). \tag{S17}$$

Remarkably, $P(\text{err}|\chi_n)$ depends only on the length $n$ of the measurement string $\chi_n$ and is a monotonic decreasing function. For a pre-set $\varepsilon$ the smallest $n_\varepsilon$ for which $P(\text{err}|\chi_{n_\varepsilon}) \leq \varepsilon$ condition is satisfied is equal to

$$n_\varepsilon = \left\lceil \frac{\ln(\varepsilon - \varepsilon^2) - \ln(q_1 q_2)}{2\ln(\cos 2\theta)} \right\rceil, \tag{S18}$$

which is exactly the cost function $C^{\text{LOL}}(\varepsilon)$

*3. Unbiased measurement.* In the UBM protocol, a fixed-angle Helstrom measurement is performed on each individual copy of the quantum system. As in every fixed-angle local measurement, each individual result is statistically independent on the measurement on other copies. While in FBM a single $D = 2$ measurement outcome concludes the run, UBM relies on the "majority vote", meaning that the final result depends only on the difference between the number of $D = 1$ and $D = 2$ outcomes and not the order these outcomes appear in a measurement. In the symmetric $q_1 = q_2$ case, the posterior probability $p_n(\psi_j|\chi_n^m)$ is a function of the random integer-valued variable $R_n = 2m - n$

$$\begin{aligned} p_n(\psi_1|\chi_n^m) &= f(R_n) = \left[1 + \left(\frac{1-\sin 2\theta}{1+\sin 2\theta}\right)^{R_n}\right]^{-1}, \\ p_n(\psi_2|\chi_n^m) &= f(-R_n) = \left[1 + \left(\frac{1+\sin 2\theta}{1-\sin 2\theta}\right)^{R_n}\right]^{-1}. \end{aligned} \tag{S19}$$

The measurement run concludes once we reach the condition $1 - f(R_n) < \varepsilon$ (or $1 - f(-R_n) < \varepsilon$) which corresponds to the outcome $|\psi_1\rangle$ (or $|\psi_2\rangle$). $1 - f(r)$ is a monotonically decreasing function, so there exists such $r_\varepsilon : 1 - f(r_\varepsilon) \leq \varepsilon)$ that will satisfy the condition for the protocol termination,

$$r_\varepsilon = \left\lceil \frac{\ln\varepsilon - \ln(1-\varepsilon)}{\ln(1-\sin 2\theta) - \ln(1+\sin 2\theta)} \right\rceil. \tag{S20}$$

We can describe the discrimination process as a discrete-time random walk for $R_n$ on the integers, with the transition probabilities given by

$$\begin{aligned} t_r &= P(R_{n+1} = r-1 | R_n = r) = \frac{1}{2}(1+\sin 2\theta) - \sin 2\theta f(r), \\ s_r &= P(R_{n+1} = r+1 | R_n = r) = \frac{1}{2}(1-\sin 2\theta) + \sin 2\theta f(r), \end{aligned} \tag{S21}$$

$C^{\text{UBM}}(\varepsilon)$ can be then calculated as the average number of steps, required to reach the absorbing boundary $R = \pm r_\varepsilon$, starring from $R_0 = 0$. According to [3], we can obtain $C^{\text{UBM}}(\varepsilon)$ as

$$C^{\text{UBM}}(\varepsilon) = \sum_{j=1}^{2r_\varepsilon - 1} b_{r_\varepsilon j} \tag{S22}$$

with

$$b_{ij} = \frac{\left[\sum_{k=0}^{i-1}(\prod_{u=1}^{i-k-1} t_{u-r_\varepsilon})(\prod_{s=i-k}^{i-1} s_{v-r_\varepsilon})\right]\left[\prod_{k=i}^{i-1} s_{k-r_\varepsilon}\right]\left[\sum_{k=0}^{2r_\varepsilon-j-1}(\prod_{u=j+1}^{2r_\varepsilon-k-1} t_{u-r_\varepsilon})(\prod_{v=2r_\varepsilon-k}^{2r_\varepsilon-1} s_{v-r_\varepsilon})\right]}{\sum_{k=0}^{2r_\varepsilon-1}(\prod_{u=1}^{2r_\varepsilon-k-1} t_{u-r_\varepsilon})(\prod_{v=2r_\varepsilon-k}^{2r_\varepsilon-1} s_{v-r_\varepsilon})}$$

for $1 \le i \le j \le n-1$ and

$$b_{ij} = \frac{\left[\sum_{k=0}^{j-1}(\prod_{u=1}^{j-k-1} t_{u-r_\varepsilon})(\prod_{v=j-k}^{j-1} s_{v-r_\varepsilon})\right]\left[\prod_{k=j+1}^{i} t_{k-r_\varepsilon}\right]\left[\sum_{k=0}^{2r_\varepsilon-i-1}(\prod_{u=i+1}^{2r_\varepsilon-k-1} t_{u-r_\varepsilon})(\prod_{v=2r_\varepsilon-k}^{2r_\varepsilon-1} s_{v-r_\varepsilon})\right]}{\sum_{k=0}^{2r_\varepsilon-1}(\prod_{u=1}^{2r_\varepsilon-k-1} t_{u-r_\varepsilon})(\prod_{v=2r_\varepsilon-k}^{2r_\varepsilon-1} s_{v-r_\varepsilon})}$$

for $n-1 \ge i > j \ge 1$.

## II. OPTIMAL MEASUREMENT ANGLES AND ASYMPTOTIC BEHAVIOR

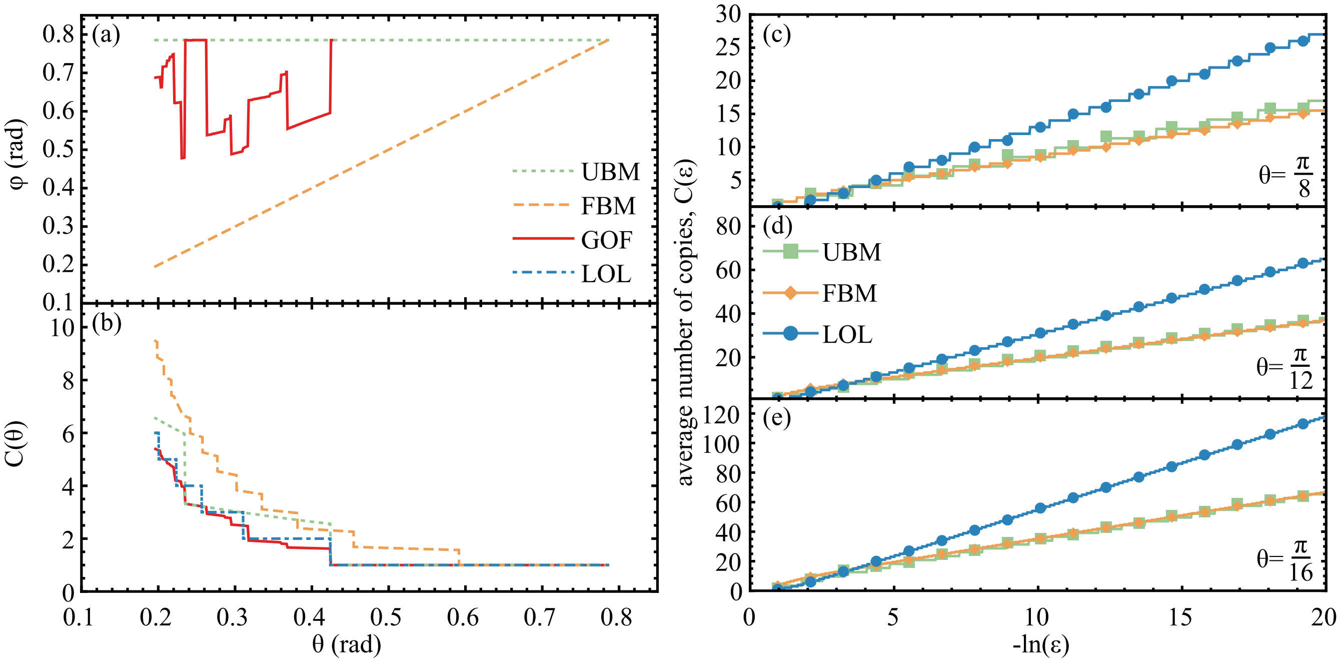


Supplemental Figure 1. (a) Measurement angles for the three fixed-angle strategies considered in this work, as function of state angle $\theta$. Here $q_1 = q_2 = 0.5$ and the error bound is set to $\varepsilon = 0.125$. (b) Corresponding average number of copies required for the GOF protocol to reach the error bound. For states with $\theta \ge 0.4249$ rad, the average number of copies required for the discrimination reaches 1. In this case there are multiple angles that can provide satisfactory discrimination error, so the optimal angle of the GOF protocol is not shown for this range of $\theta$ values. (c)-(e) Asymptotic behavior of the cost function $C(\varepsilon)$ for the UBM, FBM and LOL strategies, with $q_1 = q_2$ and state angles (c) $\theta = \pi/8$, (d) $\theta = \pi/12$ and (e) $\theta = \pi/16$.

Fig. 3 provides experimental results for the error bounds down to $\varepsilon = 0.01$ ($-\ln(\varepsilon) \approx 4.6$). For the case of very small $\varepsilon$ detailed investigation of the GOF strategy becomes computationally unfeasible. The GOF strategy, however, represents the optimal guaranteed bounded error fixed-angle approach, so comparing LOL strategy with other fixed-angle strategies should be enough to bound the asymptotic behavior of the GOF protocol. Results for the UBM, FBM and LOL strategies for error bounds down to $\varepsilon \approx 2 * 10^{-9}$ are shown in Supplemental Figure 1(c)-(e). All three strategies can be approximated by linear equation $C^{\$}(\varepsilon) = C_{\$} - \xi_{\$} \ln(\varepsilon)$, where \$ stands for UBM, FBM or LOL. Using Eq. 2, Eq. 4 and some numerical calculation we obtain that for the $q_1 = q_2$ case $\xi_{\mathrm{LOL}} \approx 2\xi_{\mathrm{FBM}}$, and more generally

$$\xi_{\mathrm{LOL}} \simeq \frac{1}{2\ln(\cos 2\theta)}, \xi_{\mathrm{FBM}} \simeq \frac{\min\{q_1, q_2\}}{2\ln(\cos 2\theta)}. \tag{S23}$$

This guarantees that the GOF strategy outperforms the adaptive LOL in the asymptotic case of small $\varepsilon$.

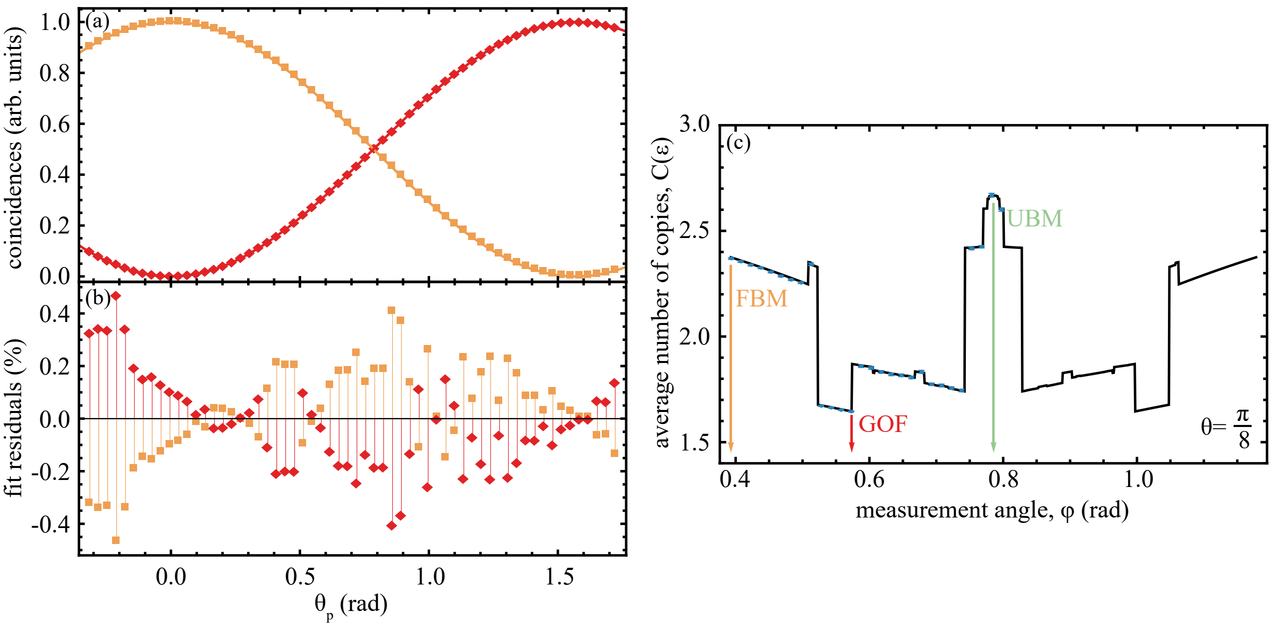


Supplemental Figure 2. Experimental state preparation and measurement characterization. (a) Normalized coincidence counts in the measurement outputs. Filled squares (■) correspond to the $|x\rangle$ projection and filled diamonds (♦) correspond to $|y\rangle$ projection. (b) - corresponding fit residuals. The standard deviation from the ideal measurement outcome is $\approx 0.177\%$. (c) Average number of copies $C(\varepsilon)$ required to perform a state discrimination with a probability of error bounded by $\varepsilon = 0.125$, as a function of measurement angle $\varphi$, for $q_1 = q_2$ and $\theta = \pi/8$. The line represents the theoretical prediction from Fig. 1(a) and points represent the experimental data.

## III. STATE CHARACTERIZATION

The experimental verification of the GOF protocol requires precise preparation of high purity linearly polarized states of arbitrary state angle $\theta$ and a high-contrast projection in the $|x\rangle, |y\rangle$ measurement basis. Quantum state tomography [4, 5] is a standard way to measure and characterize a quantum state, but it relies on the use of wave plates, when a polarization state is measured. These are usually fabricated with lower precision compared to polarizing beam displacers and high-contrast linear plate polarizers (LPP), that were used in our experiment. In order to verify the precision of our state preparation without tomography, we have used our experimental setup to prepare and measure states with $\theta = [-0.3, 1.7]$ rad, covering the whole range required for the experimental demonstration. Collected coincidence, converted into probabilities, were then compared to theoretically expected values, given by $\sin^2(\theta)$, as shown in Supplemental Figure 2(a)-(b). Additionally, we have performed fixed angle discrimination measurement for state probabilities $q_1 = q_2$, state angle $\theta = \pi/8$ and error bound $\varepsilon = 0.125$ (see theoretical prediction in Fig. 1(a)) and varying measurement angle $\varphi$. Our results, shown in Supplemental Figure 2(c), confirm precision of the experimental setup, and correctness of our choice of optimal GOF angle $\varphi^{\rm opt}$.


[1] B. L. Higgins, A. C. Doherty, S. D. Bartlett, G. J. Pryde, and H. M. Wiseman, Phys. Rev. A **83**, 052314 (2011).

[2] B. L. Higgins, B. M. Booth, A. C. Doherty, S. D. Bartlett, H. M. Wiseman, and G. J. Pryde, Phys. Rev. Lett. **103**, 220503 (2009).

[3] G. Rudolph, *The Fundamental Matrix of the General Random Walk with Absorbing Boundaries*, Tech. Rep. CI-75/99 (Department of Computer Science, University of Dortmund, 1999).

[4] D. F. V. James, P. G. Kwiat, W. J. Munro, and A. G. White, Phys. Rev. A **64**, 052312 (2001).

[5] A. G. White, A. Gilchrist, G. J. Pryde, J. L. O'Brien, M. J. Bremner, and N. K. Langford, J. Opt. Soc. Am. B **24**, 172 (2007).
